# Supplementary material for: Nontrivial temperature dependence of ferromagnetic resonance frequency for spin reorientation transitions
Source: arXiv:2009.08581 source file (2020-09-18)
Supplement: Supplementary file 1 [file Supplemental_material_FMR.pdf]

# Supplemental Material for Nontrivial temperature dependence of ferromagnetic resonance frequency for spin reorientation transitions

Masamichi Nishino[1,2] and Seiji Miyashita[3,2]

[1] *Research Center for Advanced Measurement and Characterization, Tsukuba, Ibaraki 305-0047, Japan*

[2] *Elements Strategy Initiative Center for Magnetic Materials, National Institute for Materials Science, Tsukuba, Ibaraki 305-0047, Japan*

[3] *Department of Physics, Graduate School of Science, The University of Tokyo, Bunkyo-Ku, Tokyo 113-0033, Japan*

## Magnetic anisotropy energies for the Nd magnet model

Figure S1 illustrates $\theta$ dependence of $D_1^{\rm Nd}(J_i^z)^2$, $D_2^{\rm Nd}(J_i^z)^4$, $D_3^{\rm Nd}(J_i^z)^6$, and their sum. A magnified graph for the sum is given in Fig. 1 (b) in the text. The anisotropy energies $-D_i(s_i^z)^2$ of Fe atoms are between $-12.4$ K and 24.8 K (mostly negative) and are much smaller. The contribution of the first term ($D_1^{\rm Nd}(J_i^z)^2$) is small and the competition between the second ($D_2^{\rm Nd}(J_i^z)^4$) and third ($D_3^{\rm Nd}(J_i^z)^6$) terms is important for the SR transition. Because the minimum of the potential for the sum is realized at $\theta \simeq 0.2\pi$, the spins align tilted from the c axis in the ground state. However, the order $m_{xy}^2$ in the xy plane is broken by thermal fluctuation above the SR transition, and the magnetization becomes parallel to the c-axis.

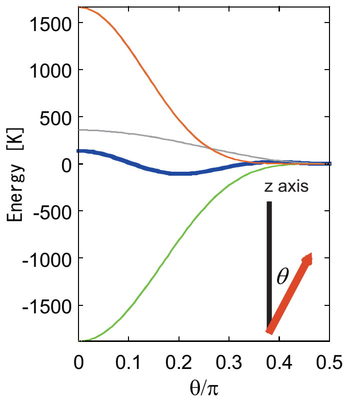


Figure 1: (color online) $\theta$ dependence of $D_1^{\rm Nd}(J_i^z)^2$ (gray), $D_2^{\rm Nd}(J_i^z)^4$ (green), $D_3^{\rm Nd}(J_i^z)^6$ (red), and their sum (blue thick) in Eq. (2) for the Nd magnet model (1).

## Temperature dependence of $\bar{I}(f)$ for the Nd magnet model

The temperature dependences of $\bar{I}(f)$ for the Nd magnet model are given in Fig. S2. We find that $f_{\rm R}$ varies non-monotonically with temperature. At low temperatures below $T_{\rm R}$, $f_{\rm R} \sim 0$ (see also Fig. 2 in the text). It increases up to around 300 K and then decreases at higher temperatures. Here the linewidths indicate the deviation of the precession frequency, i.e., FMR frequency, and we find larger deviation at higher temperatures.

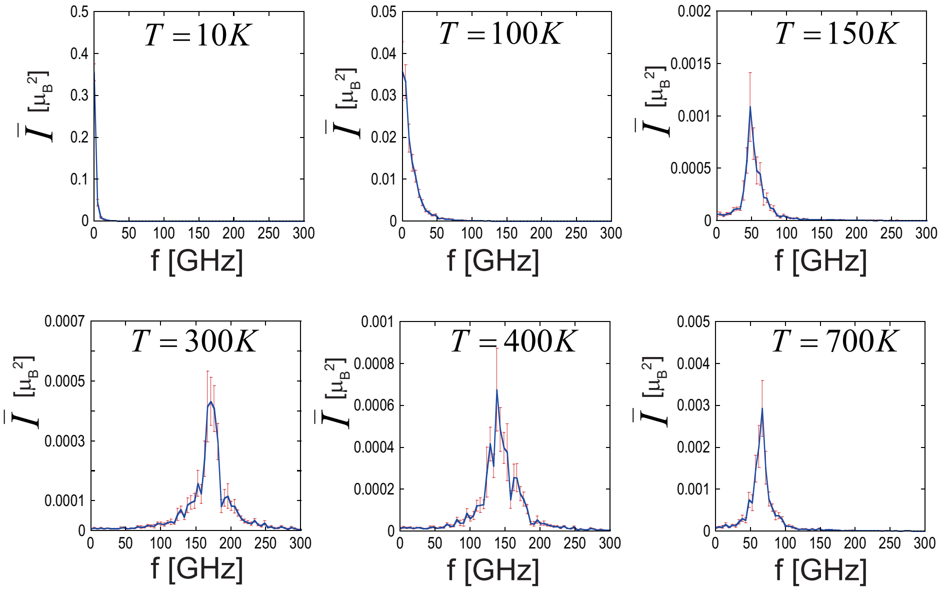


Figure 2: (color online) Temperature dependence of $\bar{I}(f)$ for the Nd magnet model (1).

**Magnetic anisotropy energies for the minimal model**

We show, in Fig. S3 (a), $\theta$ dependence of $-D_1(S^z)^2$, $-D_2(S^z)^4$, and their sum for the minimal model (6). A magnified graph for the sum is given in Fig. S3 (b). The parameters are set as $D_1 = 1$ and $D_2 = -0.7$. We see a similar potential minimum as in the Nd magnet model.

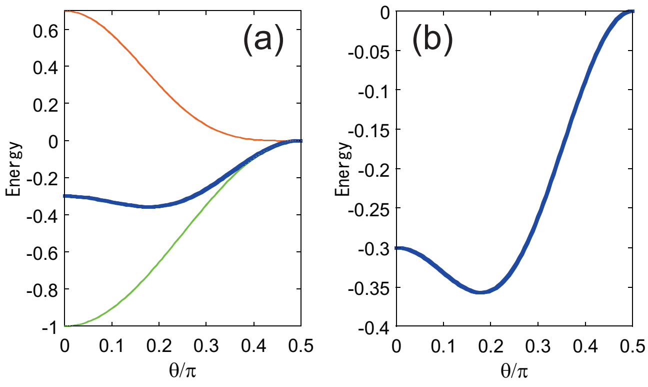


Figure 3: (color online) (a) $\theta$ dependence of $-D_1(S^z)^2$ (green), $-D_2(S^z)^4$ (red), and their sum (blue thick). $D_1 = 1$ and $D_2 = -0.7$ are set. (b) Magnified graph for the sum (blue).

**Temperature dependence of $\bar{I}(f)$ for the minimal model**

The temperature dependence of $\bar{I}(f)$ for the minimal model (6) with $D_2 = 0$ is shown in Fig. S4. We see a monotonic temperature dependence of the peak position, in which $f_{\rm R}$ shifts to lower frequency side with rising temperature. It is conventional behavior of simple ferromagnets.

The temperature dependence of $\bar{I}(f)$ for the minimal model (6) with $D_2 = -0.7$ is plotted in Fig. S5. We find non-monotonic temperature dependence of the peak position.

For $T < T_{\rm R} \simeq 0.4$, $f_{\rm R} \sim 0$, and it increases with rising temperature up to $T \simeq 1.08$ and then decreases at higher temperatures, which is qualitatively similar to that of the Nd magnet model.

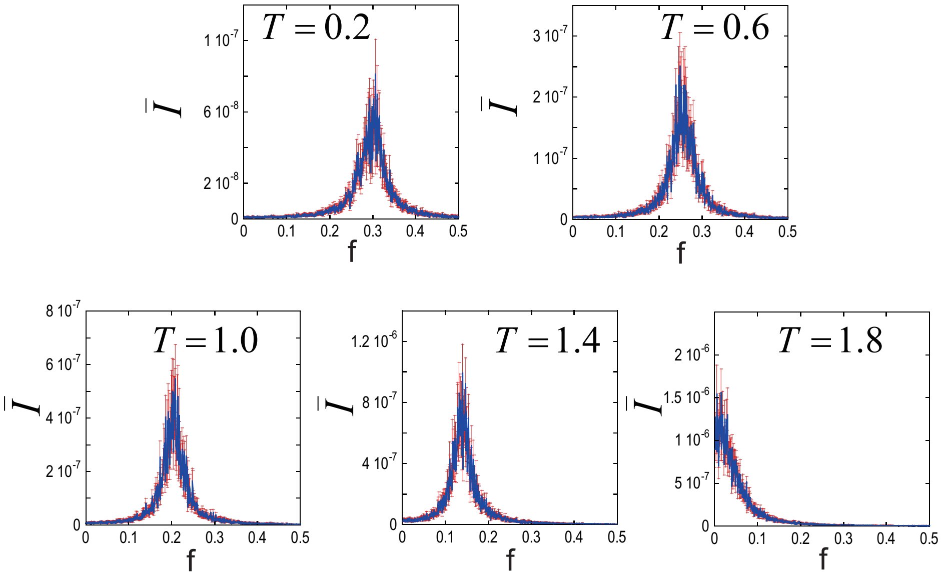


Figure 4: (color online) Temperature dependence of $\bar{I}(f)$ for the minimal model (6) with $D_2 = 0$.

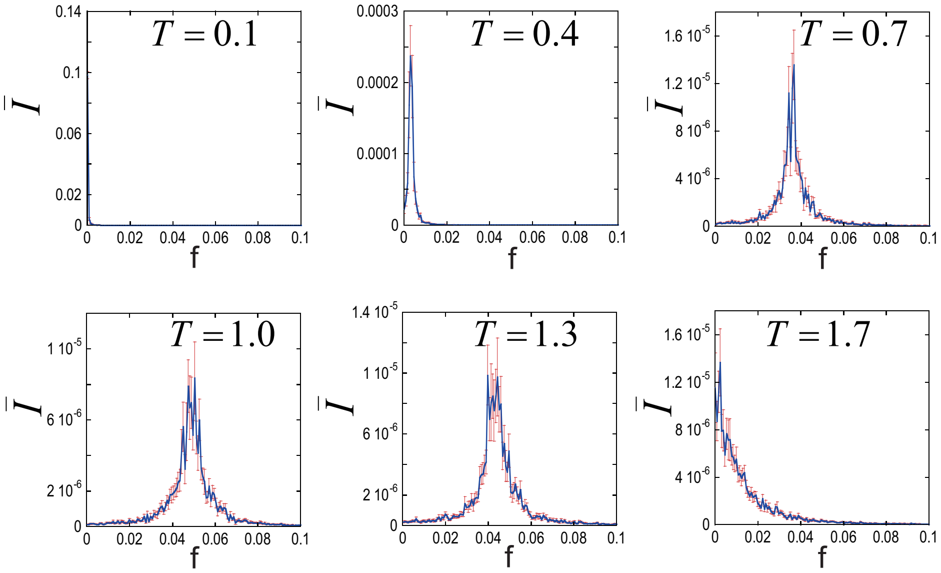


Figure 5: (color online) Temperature dependence of $\bar{I}(f)$ for the minimal model (6) with $D_2 = -0.7$.
